# Supplementary material for: Adaptive neural network classifier for decoding MEG signals
Source: arXiv:1805.10981 source file (2019-02-10)
Supplement: Supplementary file 1 [file supplementary_material.pdf]

# Supplementary material

Ivan Zubarev[a,*], Rasmus Zetter[a], Hanna-Leena Halme[a], Lauri Parkkonen[a,b]

[a] *Department of Neuroscience and Biomedical Engineering, Aalto University School of Science, FI-00076 Aalto, Finland*
[b] *Aalto NeuroImaging, Aalto University, FI-00076 Aalto, Finland*

## 1. Supplementary Tables

Table 1: Notation

| Parameter | Shape | Notation | Shape notation |
|---|---|---|---|
| Number of MEG channels | *scalar* | $n$ | |
| Number discretized time-points | *scalar* | $t$ | |
| Number of latent sources | *scalar* | $k$ | |
| Temporal filter length | *scalar* | $l$ | |
| Input shape | $204 \times 64/189$[1] | $\mathbf{X}$ | $n \times t$ |
| (De)-mixing matrix | $204 \times 32$ | $\mathbf{C}$ | $n \times k$ |
| Temporal convolution kernel | $7 \times 32(\times 32)$[2] | $\mathbf{A}$ | $l \times k(\times k)$ |

Table 2: Comparisons in across-subject classification accuracy between LF-CNN, VAR-CNN and the benchmark models in a 5-class sensory stimulation task. Statistical significance estimated using a paired t-test. * - p < 0.05; ** - p < 0.005

| | LF-CNN | | | VAR-CNN | | |
|---|---|---|---|---|---|---|
| Model | validation (%) | test (%) | test+upd (%) | validation (%) | test (%) | test+upd (%) |
| Linear-SVM | 1.68* | 2.93 | 6.26** | 2.55** | 5.72** | 7.30** |
| RBF-SVM | 1.40* | 0.36 | 9.31** | 2.28** | 3.15* | 10.3** |
| ShallowFBCSP-CNN | 9.67** | 23.0** | n.a. | 10.5** | 25.8** | n.a. |
| EEGNET-8 | 6.24** | 6.28* | 4.07** | 7.12** | 9.06** | 5.10** |
| VGG19 | 14.5** | 13.1** | 19.4** | 15.4** | 5.40** | 13.8** |

## 2. Supplementary Figures

*Corresponding author ivan.zubarev@aalto.fi

[1] Input time segment length in Experiments 1 and 2, respectively.
[2] Additional third dimension used in VAR-CNN.

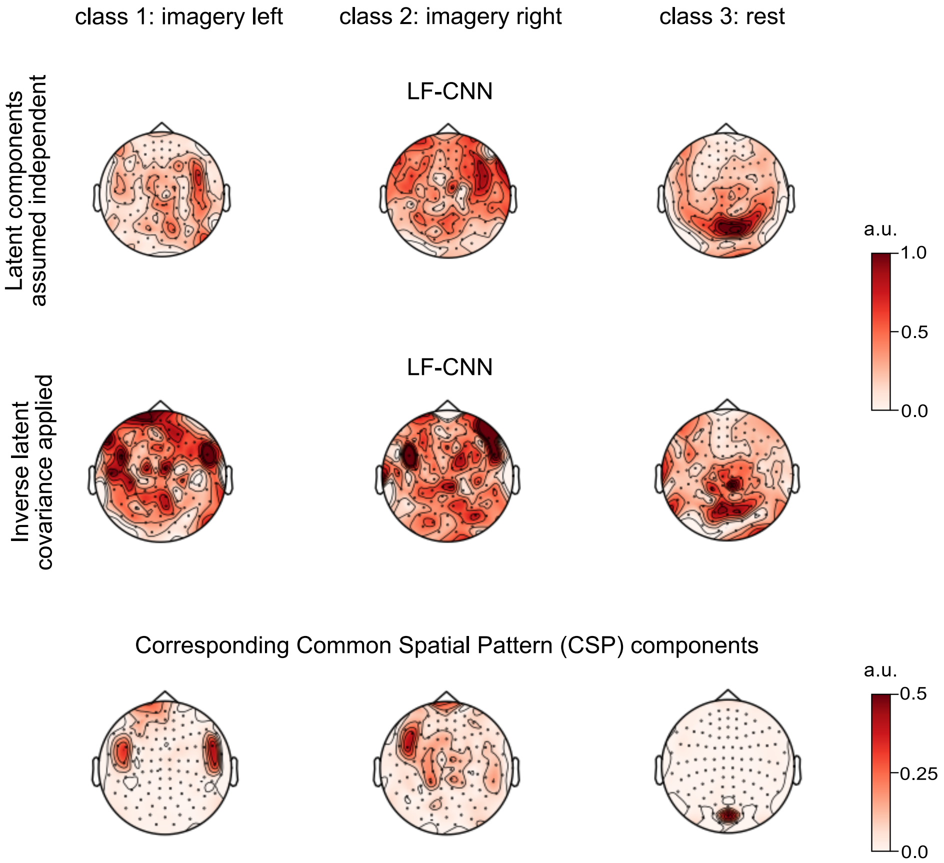


Figure 1: Spatial patterns extracted from LF-CNN model (top and middle row) and CSP (bottom row) trained on pooled data from all subjects in Experiment 2. **Top.** Spatial Patterns obtained by multiplying spatial extraction filters from the linear input layer with the covariance matrix of the data **Middle.** Spatial Patterns obtained by multiplying spatial extraction filters from the linear input layer with the (spatial) covariance matrix of the data and the inverse of the covariance matrix of the latent components. **Bottom.** Corresponding spatial patterns obtained using the Common Spatial Pattern (CSP) approach.

Table 3: Comparisons in across-subject classification accuracy between LF-CNN, VAR-CNN and the benchmark models in a 3-class motor imagery task. Statistical significance estimated using a paired t-test. * - $p < 0.05$; ** - $p < 0.005$

| | LF-CNN | | | VAR-CNN | | |
|---|---|---|---|---|---|---|
| Model | validation (%) | test (%) | test+upd (%) | validation (%) | test (%) | test+upd (%) |
| Linear-SVM | 7.52** | 6.03** | 8.58** | 9.83** | 8.37** | 10.89** |
| RBF-SVM | 4.13** | 0.20 | 6.31** | 6.44** | 2.54* | 8.62** |
| ShallowFBCSP-CNN | 20.57** | 20.31** | n.a. | 22.87** | 22.66** | n.a. |
| EEGNET-8 | 3.73** | 2.17 | −0.94 | 6.03** | 4.51** | 1.38* |
| VGG19 | 13.33** | 14.25** | 23.29** | 15.64** | 16.59** | 25.60** |
